# Supplementary material for: Game-Theoretic Malware Detection
Source: arXiv:2012.00817 source file (2022-01-07)
Supplement: Supplementary file 1 [file Appendix.tex]

\appendix
\section{Appendix}
